# Supplementary material for: DiffPINN: Generative diffusion-initialized physics-informed neural networks for accelerating seismic wavefield representation
Source: arXiv:2506.00471 source file (2025-05-31)
Supplement: Supplementary file 1 [file Appendix.tex]

\section{\textsc{SUPPLEMENTARY INFORMATION}}
% \vspace{8pt} \\ 
Supporting information for section X
